# Supplementary material for: A Longitudinal Analysis of University Rankings
Source: arXiv:1908.10632 source file (2020-01-20)
Supplement: Supplementary file 1 [file 5_appendix.tex]

\begin{appendices}

\begin{textblock}{0.43}[0,0](-0.27,-0.04)
\section{A. Results of Principal Component Analysis}\label{appx: PCA}
\end{textblock}

\begin{textblock}{0.43}[0,0](-0.27,0.01)

\begin{table}[h]
\caption{PCA Loadings on Components 2012}
\centering
\label{table:loadings2012}
\begin{tabularx}{\columnwidth}{lYYY}
\toprule
    Measure & PC1 & PC2 & PC3 \\ \midrule
    \textbf{ARWU} & & & \\
    1. Alumni  & \textbf{-0.58}  &  0.09  & \\ 
    2. Award   & \textbf{-0.46}  &  0.06  & \\ 
    3. HiCi    & \textbf{-0.60}  & -0.04  & \\ 
    4. NS      & \textbf{-0.50}  & -0.16  & \\ 
    5. PUB     &  0.00  & \textbf{-0.87}  & \\ [1.5ex]
    
    \textbf{THE} & & & \\
    1. Teaching               & \textbf{-0.93}  & -0.04  &  \\ 
    2. Research               & \textbf{-0.96}  & -0.04  &  \\ 
    3. Citations              & \textbf{-0.57}  &  \textbf{0.61}  &  \\ 
    4. Industry Income        & \textbf{-0.40}  & \textbf{-0.73}  &  \\ 
    5. International Outlook  & -0.14  &  \textbf{0.57}  &  \\ [1.5ex]
    
    \textbf{QS} & & & \\
    1. Academic reputation    & \textbf{-0.93}  &  0.00  & -0.05 \\
    2. Employer reputation    & \textbf{-0.70}  & -0.25  & -0.15  \\
    3. Faculty Student        & -0.01  &  0.03  & \textbf{-0.99}  \\
    4. International Faculty  &  0.02  & \textbf{-0.95}  &  0.10  \\
    5. International Student  & -0.02  & \textbf{-0.94}  & -0.06  \\
    6. Citations              & \textbf{-0.77}  &  0.15  &  0.18  \\
\bottomrule
\multicolumn{4}{l}{Note: Loadings larger than .40 are in bold} \\
\end{tabularx}
\end{table}
\vspace{5mm}
\begin{table}[h]
\caption{PCA Loadings on Components 2014}
\centering
\label{table:loadings2014}
\begin{tabularx}{\columnwidth}{lYYY}
\toprule
    Measure & PC1 & PC2 & PC3 \\ \midrule
    \textbf{ARWU} & & & \\
    1. Alumni  &  0.11  &  \textbf{0.64}  &  \\ 
    2. Award   &  0.02  &  \textbf{0.47}  &  \\ 
    3. HiCi    & -0.33  &  \textbf{0.42}  &  \\ 
    4. NS      & -0.28  &  \textbf{0.45}  &   \\ 
    5. PUB     & \textbf{-0.88}  & -0.01  &   \\ [1.5ex]
    
    \textbf{THE} & & & \\
    1. Teaching               & \textbf{-0.79}  & -0.06  &  \\ 
    2. Research               & \textbf{-0.85}  & -0.03  &  \\ 
    3. Citations              & \textbf{-0.49}  &  \textbf{0.60}  &   \\ 
    4. Industry Income        & -0.35  & \textbf{-0.76}  &  \\ 
    5. International Outlook  & -0.21  &  \textbf{0.59}  &  \\ [1.5ex]
    
    \textbf{QS} & & & \\
    1. Academic reputation    & \textbf{-0.93}  &  0.10  & -0.17  \\
    2. Employer reputation    & \textbf{-0.94}  & -0.11  &  0.15   \\
    3. Faculty Student        &  0.04  & -0.01  & \textbf{-0.87}   \\
    4. International Faculty  &  0.03  & \textbf{-0.96}  &  0.01   \\
    5. International Student  & -0.03  & \textbf{-0.94}  & -0.04 \\
    6. Citations              & -0.19  & -0.13  & \textbf{-0.58}  \\
\bottomrule
\multicolumn{4}{l}{Note: Loadings larger than .40 are in bold} \\
\end{tabularx}
\end{table}

\end{textblock}

\begin{textblock}{0.43}[0,0](0.2,0.01)

\begin{table}[h]
\caption{PCA Loadings on Components 2013}
\centering
\label{table:loadings2013}
\begin{tabularx}{\columnwidth}{lYYY}
\toprule
    Measure & PC1 & PC2 & PC3 \\ \midrule
    \textbf{ARWU} & & & \\
    1. Alumni  & \textbf{-0.58}  &  0.09  &   \\ 
    2. Award   & \textbf{-0.45}  &  0.04  &   \\ 
    3. HiCi    & \textbf{-0.62}  & -0.01  &  \\ 
    4. NS      & \textbf{-0.52}  & -0.16  &   \\ 
    5. PUB     &  0.00  & \textbf{-0.88}  &   \\ [1.5ex]
    
    \textbf{THE} & & & \\
    1. Teaching               & \textbf{-0.70}  & -0.22  &  \\ 
    2. Research               & \textbf{-0.75}  & -0.23  &   \\ 
    3. Citations              & \textbf{-0.68}  & \textbf{ 0.44}  &  \\ 
    4. Industry Income        & -0.19  & \textbf{-0.82}  &   \\ 
    5. International Outlook  & -0.38  &  \textbf{0.54}  &  \\ [1.5ex]
    
    \textbf{QS} & & & \\
    1. Academic reputation    & \textbf{-0.98}  &  0.08  & -0.09   \\
    2. Employer reputation    & \textbf{-0.90}  & -0.12  &  0.13   \\
    3. Faculty Student        &  0.03  & -0.02  & \textbf{-0.94}   \\
    4. International Faculty  &  0.03  & \textbf{-0.97}  &  0.03 \\
    5. International Student  & -0.03  & \textbf{-0.94}  & -0.05  \\
    6. Citations              & -0.38  & -0.08  & \textbf{-0.43}  \\
\bottomrule
\multicolumn{4}{l}{Note: Loadings larger than .40 are in bold} \\
\end{tabularx}
\end{table}
\vspace{5mm}
\begin{table}[h]
\caption{PCA Loadings on Components 2015}
\centering
\label{table:loadings2015}
\begin{tabularx}{\columnwidth}{lYYY}
\toprule
    Measure & PC1 & PC2 & PC3  \\ \midrule
    \textbf{ARWU} & & & \\
    1. Alumni  & \textbf{-0.63 } &  0.14  &   \\ 
    2. Award   & \textbf{-0.48}  &  0.04  &   \\ 
    3. HiCi    & \textbf{-0.47}  & -0.27  &  \\ 
    4. NS      & \textbf{-0.50}  & -0.22  &  \\ 
    5. PUB     &  0.00  & \textbf{-0.87}  &   \\ [1.5ex]
    
    \textbf{THE} & & & \\
    1. Teaching               & \textbf{-0.41}  & \textbf{-0.40}  &   \\ 
    2. Research               & \textbf{-0.50}  & \textbf{-0.44}  &   \\ 
    3. Citations              & \textbf{-0.86}  & -0.13  &  \\ 
    4. Industry Income        &  0.05  & \textbf{-1.00}  & \\ 
    5. International Outlook  & \textbf{-0.88}  &  0.22  &  \\ [1.5ex]
    
    \textbf{QS} & & & \\
    1. Academic reputation    & \textbf{-0.94}  & -0.06  & -0.01  \\
    2. Employer reputation    & \textbf{-0.93}  &  0.10  &  0.08   \\
    3. Faculty Student        &  0.00  &  0.02  & \textbf{-0.99}   \\
    4. International Faculty  &  0.02  & \textbf{ 0.89}  &  0.00   \\
    5. International Student  & -0.02  &  \textbf{1.00}  & -0.02  \\
    6. Citations              & \textbf{-0.69}  & -0.07  & -0.25  \\
\bottomrule
\multicolumn{4}{l}{Note: Loadings larger than .40 are in bold} \\
\end{tabularx}
\end{table}

\end{textblock}

\clearpage

\begin{textblock}{0.43}[0,0](-0.27,0)

\begin{table}[h]
\caption{PCA Loadings on Components 2016}
\centering
\label{table:loadings2016}
\begin{tabularx}{\columnwidth}{lYYY}
\toprule
    Measure & PC1 & PC2 & PC3  \\ \midrule
    \textbf{ARWU} & & & \\
    1. Alumni  &  0.05  &  \textbf{0.67}  &  \\ 
    2. Award   & -0.04  &  \textbf{0.46}  &  \\ 
    3. HiCi    & \textbf{-0.63}  &  0.04  &   \\ 
    4. NS      & -0.37  &  0.37  &   \\ 
    5. PUB     & \textbf{-0.85}  & -0.03  &  \\ [1.5ex]
    
    \textbf{THE} & & & \\
    1. Teaching               & -0.33  & \textbf{-0.47}  & \\ 
    2. Research               & \textbf{-0.46}  & \textbf{-0.47}  &   \\ 
    3. Citations              & \textbf{-0.85}  & -0.21  &   \\ 
    4. Industry Income         &  0.08  & \textbf{-0.90}  &  \\ 
    5. International Outlook  & \textbf{-0.96}  &  0.19  &   \\ [1.5ex]
    
    \textbf{QS} & & & \\
1. Academic reputation    & \textbf{-0.61}  &  0.04  &  \textbf{0.59}  \\
2. Employer reputation    & \textbf{-0.67}  & -0.16  &  0.35   \\
3. Faculty Student        & \textbf{-0.93}  &  0.01 & -0.20 \\
4. International Faculty  &  0.11  & \textbf{-0.95}  &  0.04  \\
5. International Student  & -0.12  & \textbf{-0.93}  & -0.05  \\
6. Citations              &  0.09  & -0.04  &  \textbf{0.96}   \\

\bottomrule
\multicolumn{4}{l}{Note: Loadings larger than .40 are in bold} \\
\end{tabularx}
\end{table}
\vspace{5mm}
\begin{table}[h]
\caption{PCA Loadings on Components 2018}
\centering
\label{table:loadings2018}
\begin{tabularx}{\columnwidth}{lYYY}
\toprule
    Measure & PC1 & PC2 & PC3 \\ \midrule
    \textbf{ARWU} & & & \\
    1. Alumni  &  0.04  &  \textbf{0.66}  &   \\ 
    2. Award   & -0.03  &  \textbf{0.48}  &  \\ 
    3. HiCi    & \textbf{-0.66}  & -0.02  &   \\ 
    4. NS      & -0.36  &  0.35  &   \\ 
    5. PUB     & \textbf{-0.84}  & -0.01  &  \\ [1.5ex]
    
    \textbf{THE} & & & \\
    1. Teaching               & -0.28  & \textbf{-0.45}  &  \\ 
    2. Research               & \textbf{-0.42}  & \textbf{-0.45}  &  \\ 
    3. Citations              & \textbf{-0.89}  & -0.12  &   \\
    4. Industry Income         &  0.07  & \textbf{-0.88}  &   \\ 
    5. International Outlook  & \textbf{-0.96}  &  0.12  & \\ [1.5ex]
    
    \textbf{QS} & & & \\
    1. Academic reputation    & \textbf{-0.99}  & -0.05  &  0.03   \\
    2. Employer reputation    & \textbf{-0.92}  &  0.04  &  0.10  \\
    3. Faculty Student        & -0.15  &  0.04  &  \textbf{0.92}   \\
    4. International Faculty  &  0.01  &  \textbf{0.94}  & -0.08  \\
    5. International Student  &  0.02  &  \textbf{0.95}  &  0.10   \\
    6. Citations              & \textbf{-0.55}  &  0.14  & \textbf{-0.58}  \\
\bottomrule
\multicolumn{4}{l}{Note: Loadings larger than .40 are in bold} \\
\end{tabularx}
\end{table}

\end{textblock}

\begin{textblock}{0.43}[0,0](0.2,0)

\begin{table}[h]
\caption{PCA Loadings on Components 2017}
\centering
\label{table:loadings2017}
\begin{tabularx}{\columnwidth}{lYYY}
\toprule
    Measure & PC1 & PC2 & PC3 \\ \midrule
    \textbf{ARWU} & & & \\
    1. Alumni  &  0.03  &  \textbf{0.67}  &   \\
    2. Award   & -0.05  &  \textbf{0.47}  &  \\ 
    3. HiCi    & \textbf{-0.69}  & -0.08  & \\ 
    4. NS      & \textbf{-0.40}  &  0.30  &  \\
    5. PUB     & \textbf{-0.78}  &  0.03  &  \\ [1.5ex]
    
    \textbf{THE} & & & \\
    1. Teaching               & -0.35  & \textbf{-0.40}  & \\ 
    2. Research               & \textbf{-0.47}  & \textbf{-0.43}  & \\ 
    3. Citations              & \textbf{-0.89}  & -0.11  & \\ 
    4. Industry Income         &  0.05  & \textbf{-0.95}  & \\ 
    5. International Outlook  & \textbf{-0.95}  &  0.14  &  \\ [1.5ex]
    
    \textbf{QS} & & & \\
    1. Academic reputation    & \textbf{-0.90}  &  0.08  & -0.27   \\
    2. Employer reputation        & \textbf{-0.76}  & -0.13  & -0.34   \\
    3. Faculty Student & -0.10  & -0.03  & \textbf{-0.92}   \\
    4. International Faculty  &  0.02  & \textbf{-0.92}  & -0.01   \\
    5. International Student              &  0.00  & \textbf{-0.95}  &  0.00  \\
    6. Citations    & \textbf{-0.88}  & -0.06  &  \textbf{0.46}   \\
\bottomrule
\multicolumn{4}{l}{Note: Loadings larger than .40 are in bold} \\
\end{tabularx}
\end{table}

\end{textblock}

\clearpage

\begin{textblock}{0.43}[0,0](-0.27,-0.04)
\section{B. Results of Factor Analysis} \label{appx: EFA}
\end{textblock}

\begin{textblock}{0.43}[0,0](-0.27,0.02)
\begin{table}[h]
\caption{NIPA Loadings on Factors 2012}
\centering
\label{table:loadings2012}
\begin{tabularx}{\columnwidth}{lYYY}
\toprule
    Measure & PA1 & PA2 & PA3 \\ \midrule
    \textbf{ARWU} & & & \\
    1. Alumni    & 0.04  & \textbf{ 0.79}  & \\ 
    2. Award     & 0.01  &  \textbf{0.85}  & \\ 
    3. HiCi      & \textbf{0.82}  &  0.07  & \\ 
    4. NS       & \textbf{0.81}  &  0.14  & \\ 
    5. PUB      & \textbf{0.83}  & -0.15  & \\ [1.5ex]
    
    \textbf{THE} & & & \\
    1. Teaching                & \textbf{0.94}  &  0.01  & \\ 
    2. Research                 & \textbf{0.95}  &  0.01  & \\ 
    3. Citations                & 0.32  &  \textbf{0.43}  & \\ 
    4. Industry Income         & 0.38  & -0.36  & \\ 
    5. International Outlook  & 0.06  &  0.25  & \\ [1.5ex]
    
    \textbf{QS} & & & \\
    1. Academic reputation     &  \textbf{0.76}  & -0.04  &  0.18 \\
    2. Employer reputation     &  \textbf{0.81}  &  0.06  & -0.12 \\
    3. Faculty Student        &  0.19  & -0.02  &  0.09 \\
    4. International Faculty & -0.05  &  \textbf{0.78}  &  0.02 \\
    5. International Student    &  0.06  &  \textbf{0.76}  &  0.00 \\
    6. Citations                &  0.16  &  0.07  &  \textbf{0.41} \\
\bottomrule
\multicolumn{4}{l}{Note: Loadings larger than .40 are in bold} \\
\end{tabularx}
\end{table}
\vspace{5mm}
\begin{table}[h]
\caption{NIPA Loadings on Factors 2014}
\centering
\label{table:loadings2014}
\begin{tabularx}{\columnwidth}{lYYY}
\toprule
    Measure  & PA1 & PA2 & PA3 \\ \midrule
    \textbf{ARWU} & & & \\
    1. Alumni  & 0.03  &  \textbf{0.80}  & \\ 
    2. Award     & 0.03  &  \textbf{0.84}  & \\ 
    3. HiCi      & \textbf{0.87}  &  0.03  & \\ 
    4. NS        & \textbf{0.75}  &  0.22  & \\ 
    5. PUB     & \textbf{0.82}  & -0.14  & \\ [1.5ex]
    
    \textbf{THE} & & & \\
    1. Teaching               & \textbf{0.94}  & -0.01  & \\ 
    2. Research                & \textbf{0.95}  &  0.02  & \\ 
    3. Citations               & 0.27  &  \textbf{0.40} & \\ 
    4. Industry Income          & 0.33  & -0.35  & \\ 
    5. International Outlook  & 0.09  &  0.31  & \\ [1.5ex]
    
    \textbf{QS} & & & \\
    1. Academic reputation    -0.17  &  \textbf{0.78}  & -0.06  &  0.22 \\
    2. Employer reputation    &  \textbf{0.82}  &  0.08  & -0.16 \\
    3. Faculty Student         &  0.15  &  0.06  &  0.11 \\
    4. International Faculty   & -0.02  &  \textbf{0.77}  &  0.00 \\
    5. International Student   &  0.03  &  \textbf{0.77}  &  0.03 \\
    6. Citations              &  0.08  &  0.15  &  \textbf{0.50} \\
\bottomrule
\multicolumn{4}{l}{Note: Loadings larger than .40 are in bold} \\
\end{tabularx}
\end{table}
\end{textblock}

\begin{textblock}{0.43}[0,0](0.2,0.02)
\begin{table}[h]
\caption{NIPA Loadings on Factors 2013}
\centering
\label{table:loadings2013}
\begin{tabularx}{\columnwidth}{lYYY}
\toprule
    Measure & PA1 & PA2 & PA3 \\ \midrule
    \textbf{ARWU} & & & \\
    1. Alumni   & 0.03  &  \textbf{0.79}  & \\ 
    2. Award    & 0.02  &  \textbf{0.84} & \\ 
    3. HiCi     & \textbf{0.81}  &  0.06  & \\ 
    4. NS       & \textbf{0.81}  &  0.14  & \\ 
    5. PUB     & \textbf{0.82}  & -0.15  & \\ [1.5ex]
    
    \textbf{THE} & & & \\
    1. Teaching                 & \textbf{0.93}  &  0.00  & \\ 
    2. Research             & \textbf{0.94}  &  0.01  & \\ 
    3. Citations               & 0.31  &  \textbf{0.40}  & \\ 
    4. Industry Income          & 0.36  & -0.34  & \\ 
    5. International Outlook    & 0.08  &  0.27  & \\ [1.5ex]
    
    \textbf{QS} & & & \\
    1. Academic reputation      &  \textbf{0.76}  & -0.05  &  0.23 \\
    2. Employer reputation     &  \textbf{0.82}  &  0.08  & -0.15 \\
    3. Faculty Student        &  0.13  &  0.04  &  0.14 \\
    4. International Faculty   & -0.03  &  \textbf{0.79}  &  0.02 \\
    5. International Student   &  0.03  &  \textbf{0.79}  &  0.01 \\
    6. Citations               &  0.09  &  0.14  &  \textbf{0.51} \\
\bottomrule
\multicolumn{4}{l}{Note: Loadings larger than .40 are in bold} \\
\end{tabularx}
\end{table}
\vspace{5mm}
\begin{table}[h]
\caption{NIPA Loadings on Factors 2015}
\centering
\label{table:loadings2015}
\begin{tabularx}{\columnwidth}{lYYY}
\toprule
    Measure & PA1 & PA2 & PA3 \\ \midrule
    \textbf{ARWU} & & & \\
    1. Alumni   & 0.04  &  \textbf{0.80}  & \\ 
    2. Award   & 0.03  &  \textbf{0.84}  & \\ 
    3. HiCi      & \textbf{0.86}  &  0.05  & \\ 
    4. NS        & \textbf{0.75}  &  0.22  & \\ 
    5. PUB      & \textbf{0.81}  & -0.16  & \\ [1.5ex]
    
    \textbf{THE} & & & \\
    1. Teaching                &  \textbf{0.95}  & -0.04  & \\ 
    2. Research                &  \textbf{0.89}  &  0.10  & \\ 
    3. Citations               &  0.22  &  \textbf{0.57}  & \\ 
    4. Industry Income         &  \textbf{0.46}  & -0.18  & \\ 
    5. International Outlook   & -0.06  &  \textbf{0.66}  & \\ [1.5ex]
    
    \textbf{QS} & & & \\
    1. Academic reputation      &  \textbf{0.87}  & -0.07  &  0.02 \\
    2. Employer reputation     &  \textbf{0.84}  &  0.07  & -0.04 \\
    3. Faculty Student       &  0.39  &  0.10  &  0.14 \\
    4. International Faculty   & -0.03  &  \textbf{0.69}  & -0.01 \\
    5. International Student   &  0.03  & \textbf{ 0.70}  &  0.01 \\
    6. Citations                &  \textbf{0.46}  & -0.01  &  0.10 \\
\bottomrule
\multicolumn{4}{l}{Note: Loadings larger than .40 are in bold} \\
\end{tabularx}
\end{table}
\end{textblock}

\clearpage

\begin{textblock}{0.43}[0,0](-0.27,0)
\begin{table}[h]
\caption{NIPA Loadings on Factors 2016}
\centering
\label{table:loadings2016}
\begin{tabularx}{\columnwidth}{lYYY}
\toprule
    Measure & PA1 & PA2 & PA3 \\ \midrule
    \textbf{ARWU} & & & \\
    1. Alumni    &  \textbf{0.84}  & -0.01  & \\ 
    2. Award    &  \textbf{0.84}  &  0.03  & \\ 
    3. HiCi    & -0.02  &  \textbf{0.80}  & \\ 
    4. NS       &  0.37  &  \textbf{0.60}  & \\ 
    5. PUB      & -0.07  &  \textbf{0.75}  & \\ [1.5ex]
    
    \textbf{THE} & & & \\
    1. Teaching                 &  \textbf{0.95}  & -0.04  & \\ 
    2. Research                 &  \textbf{0.86}  &  0.14  & \\ 
    3. Citations                &  0.24  &  \textbf{0.61}  & \\ 
    4. Industry Income           &  \textbf{0.57}  & -0.18  & \\ 
    5. International Outlook   & -0.06  & \textbf{ 0.71} & \\ [1.5ex]
    
    \textbf{QS} & & & \\
1. Academic reputation   &  \textbf{0.87}  & -0.06  &  0.07 \\
2. Employer reputation      &  \textbf{0.76}  &  0.11  & -0.07 \\
3. Faculty Student         &  \textbf{0.50}  & -0.05  & -0.20 \\
4. International Faculty   & -0.06  &  \textbf{0.73}  &  0.03 \\
5. International Student    &  0.07  &  \textbf{0.72}  & -0.02 \\
6. Citations             &  \textbf{0.40}  &  0.12  &  0.31 \\

\bottomrule
\multicolumn{4}{l}{Note: Loadings larger than .40 are in bold} \\
\end{tabularx}
\end{table}
\vspace{5mm}
\begin{table}[h]
\caption{NIPA Loadings on Factors 2018}
\centering
\label{table:loadings2018}
\begin{tabularx}{\columnwidth}{lYYY}
\toprule
    Measure & PA1 & PA2 & PA3 \\ \midrule
    \textbf{ARWU} & & & \\
    1. Alumni   &  \textbf{0.84}  & 0.00  & \\ 
    2. Award    &  \textbf{0.86}  & 0.01  & \\ 
    3. HiCi     &  0.01  & \textbf{0.79}  & \\ 
    4. NS        & \textbf{ 0.41}  & \textbf{0.58}  & \\ 
    5. PUB      & -0.09  & \textbf{0.75}  & \\ [1.5ex]
    
    \textbf{THE} & & & \\
    1. Teaching                &  \textbf{0.92}  & -0.02  & \\ 
    2. Research                &  \textbf{0.86}  &  0.15  & \\ 
    3. Citations              &  0.16  &  \textbf{0.66}  & \\
    4. Industry Income         & \textbf{0.63}  & -0.20  & \\ 
    5. International Outlook  & -0.04  &  \textbf{0.73}  & \\ [1.5ex]
    
    \textbf{QS} & & & \\
    1. Academic reputation  &   \textbf{0.88}  & -0.06  &  0.07 \\
    2. Employer reputation    &  \textbf{0.83}  &  0.08  & -0.08 \\
    3. Faculty Student        &  0.24  & -0.01  & \textbf{-0.40} \\
    4. International Faculty   & -0.02  &  \textbf{0.75}  &  0.07 \\
    5. International Student   &  0.02  &  \textbf{0.76}  & -0.06 \\
    6. Citations               &  0.26  &  0.13  &  \textbf{0.44} \\
\bottomrule
\multicolumn{4}{l}{Note: Loadings larger than .40 are in bold} \\
\end{tabularx}
\end{table}

\end{textblock}

\begin{textblock}{0.43}[0,0](0.2,0)
\begin{table}[h]
\caption{NIPA Loadings on Factors 2017}
\centering
\label{table:loadings2017}
\begin{tabularx}{\columnwidth}{lYYY}
\toprule
    Measure &  PA1 & PA2 & PA3 \\ \midrule
    \textbf{ARWU} & & & \\
    1. Alumni    &  \textbf{0.84}  & 0.00  & \\
    2. Award   &  \textbf{0.85}  & 0.03  & \\ 
    3. HiCi      & -0.04  & \textbf{0.80}  & \\ 
    4. NS        &  0.34  & \textbf{0.63}  & \\
    5. PUB      & -0.07  & \textbf{0.74}  & \\ [1.5ex]
    
    \textbf{THE} & & & \\
    1. Teaching                &  \textbf{0.94}  & -0.03  & \\ 
    2. Research                &  \textbf{0.88}  &  0.13  & \\ 
    3. Citations                &  0.20  &  \textbf{0.64}  & \\ 
    4. Industry Income          &  \textbf{0.59}  & -0.18  & \\ 
    5. International Outlook    & -0.06  &  \textbf{0.74}  & \\ [1.5ex]
    
    \textbf{QS} & & & \\
    1. Academic reputation    &  \textbf{0.87}  & -0.09  &  0.05 \\
    2. Employer reputation         &  \textbf{0.76}  &  0.14  & -0.05 \\
    3. Faculty Student  &  0.38  & -0.01  & -0.31 \\
    4. International Faculty   & -0.03  &  \textbf{0.69}  &  0.01 \\
    5. International Student             &  0.02  &  \textbf{0.68}  &  0.00 \\
    6. Citations     &  0.36  &  0.11  &  0.35 \\
\bottomrule
\multicolumn{4}{l}{Note: Loadings larger than .40 are in bold} \\
\end{tabularx}
\end{table}
\end{textblock}

\clearpage

\begin{textblock}{0.89}[0,0](-0.27,-0.05)

\section{C. Correlations between concepts} \label{appx: conceptcorrelations}
\vspace{5mm}
\begin{table}[h]
\caption{Spearman correlations between concepts}\label{concept_correlations}
\begin{tabularx}{\columnwidth}{lYYYYY}
\toprule
{} &  1 &  2 &  3 &  4 &  5 \\
\midrule

\textbf{2018} & & \\
  1. ARWU Publication &  &  &  &  &  \\ 
  2. THE Publication &  0.56*** &  &  &  &  \\ 
  3. QS Publication &  0.40*** &  0.40*** &  &  &  \\ 
  4. ARWU Reputation &  0.45*** &  0.46*** &  0.19*** &  &  \\ 
  5. THE Reputation &  0.71*** &  0.44*** &  0.53*** &  0.51*** &  \\ 
  6. QS Reputation &  0.56*** &  0.24*** &  0.34*** &  0.40*** &  0.74*** \\ 

\textbf{2017} & & \\
  1. ARWU Publication &  &  &  &  &  \\ 
  2. THE Publication &  0.69*** &  &  &  &  \\ 
  3. QS Publication &  0.40*** &  0.44*** &  &  &  \\ 
  4. ARWU Reputation &  0.64*** &  0.67*** &  0.30*** &  &  \\ 
  5. THE Reputation &  0.79*** &  0.59*** &  0.56*** &  0.59*** &  \\ 
  6. QS Reputation &  0.67*** &  0.47*** &  0.40*** &  0.49*** &  0.83*** \\

\textbf{2016} & & \\
  1. ARWU Publication &  &  &  &  &  \\ 
  2. THE Publication &  0.72*** &  &  &  &  \\ 
  3. QS Publication &  0.46*** &  0.54*** &  &  &  \\ 
  4. ARWU Reputation &  0.62*** &  0.65*** &  0.36*** &  &  \\ 
  5. THE Reputation &  0.77*** &  0.64*** &  0.56*** &  0.59*** &  \\ 
  6. QS Reputation &  0.68*** &  0.50*** &  0.46*** &  0.50*** &  0.84*** \\

\textbf{2015} & & \\
  1. ARWU Publication &  &  &  &  &  \\ 
  2. THE Publication &  0.72*** &  &  &  &  \\ 
  3. QS Publication &  0.40*** &  0.45*** &  &  &  \\ 
  4. ARWU Reputation &  0.72*** &  0.64*** &  0.39*** &  &  \\ 
  5. THE Reputation &  0.81*** &  0.67*** &  0.54*** &  0.69*** &  \\ 
  6. QS Reputation &  0.72*** &  0.48*** &  0.49*** &  0.60*** &  0.84*** \\

\textbf{2014} & & \\
  1. ARWU Publication &  &  &  &  &  \\ 
  2. THE Publication &  0.55*** &  &  &  &  \\ 
  3. QS Publication &  0.61*** &  0.60*** &  &  &  \\ 
  4. ARWU Reputation &  0.53*** &  0.52*** &  0.41*** &  &  \\ 
  5. THE Reputation &  0.72*** &  0.38*** &  0.58*** &  0.44*** &  \\ 
  6. QS Reputation &  0.53*** &  0.18** &  0.25*** &  0.36*** &  0.70*** \\ 

\textbf{2013} & & \\
  1. ARWU Publication &  &  &  &  &  \\ 
  2. THE Publication &  0.52*** &  &  &  &  \\ 
  3. QS Publication &  0.62*** &  0.58*** &  &  &  \\ 
  4. ARWU Reputation &  0.56*** &  0.53*** &  0.44*** &  &  \\ 
  5. THE Reputation &  0.70*** &  0.40*** &  0.59*** &  0.44*** &  \\ 
  6. QS Reputation &  0.53*** &  0.23*** &  0.26*** &  0.36*** &  0.68*** \\ 

\textbf{2012} & & \\
  1. ARWU Publication &  &  &  &  &  \\ 
  2. THE Publication &  0.56*** &  &  &  &  \\ 
  3. QS Publication &  0.66*** &  0.62*** &  &  &  \\ 
  4. ARWU Reputation &  0.52*** &  0.51*** &  0.41*** &  &  \\ 
  5. THE Reputation &  0.74*** &  0.45*** &  0.57*** &  0.45*** &  \\ 
  6. QS Reputation &  0.50*** &  0.25*** &  0.22*** &  0.34*** &  0.68*** \\

\bottomrule
\multicolumn{6}{l}{Note: ${}^{*} p<.05$, ${}^{**} p<.01$, ${}^{***} p<.001$ }
\end{tabularx}
\end{table}

\end{textblock}

\clearpage

\begin{textblock}{0.89}[0,0](-0.27,-0.04)
\section{D. Correlations between variables for the 2018 rankings} \label{appx: correlationsbetwwenvariables}
\end{textblock}

\begin{textblock}{0.89}[0,0](-0.27,0.01)
\begin{table*}[h]
\caption{Means, standard deviations, and correlations of variables within rankings}
\label{table: descriptives}
\noindent
\begin{tabular*}{\textwidth}{l @{\extracolsep{\fill}}@{}lld{3.3}d{5.3}d{6.5}d{5.5}d{4.5}d{3.5}d{2.5}d{1.5}@{}}
\toprule
& Measure
  & \multicolumn{1}{r}{Mean} 
  & \multicolumn{1}{c}{SD}
  & \multicolumn{6}{c@{}}{Correlations}\\
\cmidrule(l){5-10}
& & & & \multicolumn{1}{c}{1{.}}
      & \multicolumn{1}{c}{2{.}}
      & \multicolumn{1}{c}{3{.}}
      & \multicolumn{1}{c}{4{.}}
      & \multicolumn{1}{c}{5{.}}
      & \multicolumn{1}{c@{}}{6{.}}\\
\midrule
& \textbf{ARWU} \\
1{.} & Alumni &   23.54 &   18.50  \\
2{.} & Award  &   27.34 &   23.47 & 0.64  \\
3{.} & HiCi &   33.71 &  14.43 & 0.06  &  0.16  & \\
4{.} & NS & 31.93 &  15.10 & 0.46^{***}  & 0.54^{***} &  0.54^{***} \\
5{.} & PUB & 57.43 & 12.99 & 0.15  & 0.02  &  0.50^{***} & 0.45^{***} \\
6{.} & PCP & 35.09 &  13.47  & 0.24^{*}  &  0.38^{***}    &   0.37^{***}  & 0.29^{**} & -0.15 \\
7{.} & Overall Score & 36.70 &  12.87  & 0.57^{***} &  0.69^{***} &  0.61^{***} &  0.84^{***} &  0.53^{***} &  0.36^{***} \\[1.5ex]
& \textbf{THE}  \\
1{.} & Teaching       &     54.04 &     16.32  \\
2{.} & Research  &     56.12 &     18.00 &  0.82^{**}  \\
3{.} & Citations &     85.69 &     12.00 &  0.18*    &  0.17^{*} \\
4{.} & Industry Income  & 59.35 &  20.46 & 0.19^{**}   &  0.30^{***} & -0.23^{**}   \\
5{.} & International Outlook & 71.26 &  18.51 & -0.19^{**}   &  0.04     &  0.11     & -0.11 \\
6{.} & Overall Score &  69.17 & 39.30 & 0.80^{***} &  0.87^{***} &  0.48^{***} &  0.17^{*} &  0.12  \\[1.5ex]
& \textbf{QS} \\
1{.} & Academic reputation &   40.07 &   26.85  \\
2{.} & Employer reputation  &   40.38 &   28.16 & 0.76^{***}   \\
3{.} & Faculty Student &   51.99 &  30.19 & 0.08     &  0.09^{*} \\
4{.} & International Faculty & 53.98 & 34.99 &  0.19^{***} &  0.25^{***} & -0.05 \\
5{.} & International Students & 47.74 & 32.45 &  0.16^{***}  &  0.26^{***} &  0.03 &  0.67^{***} \\
6{.} & Citations & 44.19 &  26.88 & 0.41^{***} &  0.26^{***} & -0.21^{***} &  0.32^{***} &  0.24^{***} \\
7{.} & Overall Score & 44.50 &  18.66 & 0.85^{***} &  0.73^{***} &  0.32^{***} &  0.38^{***} &  0.38^{***} &  0.55^{***} \\
\bottomrule
& \multicolumn{3}{l}{Note: ${}^{*} p<.05$, 
  ${}^{**} p<.01$, 
  ${}^{***} p<.001$ } \\
\end{tabular*}
\end{table*}
\end{textblock}

\clearpage

\begin{textblock}{0.89}[0,0](-0.27,-0.05)

\section{E. Cronbach's alpha for complete ranking} \label{appx: conceptcorrelations}
\vspace{5mm}
\begin{table}[h]
\caption{Standardized Cronbach's alpha for complete ranking}\label{Cronbachs Alpha}
\begin{tabularx}{\columnwidth}{lYYY}
\toprule
{} &  ARWU &  THE &  QS \\
\midrule

\textbf{2018} &
 0.88 & 0.82 & 0.67 \\

\textbf{2017} &
 0.88 & 0.82 & 0.67 \\

\textbf{2016}  &
 0.89 & 0.82 & 0.72 \\

\textbf{2015}  &
 0.9 & 0.78 & 0.67 \\
  
\textbf{2014}  &
 0.91 & 0.62 & 0.67 \\
  
\textbf{2013}  &
  0.90 & 0.64 & 0.69 \\

\textbf{2012}  &
  0.91 & 0.64 & 0.66 \\

\bottomrule
\multicolumn{3}{l}{}
\end{tabularx}
\end{table}

\end{textblock}

\end{appendices}

\clearpage

\begin{textblock}{0.89}[0,0](-0.27,-0.04)
\section{F. Similarity between ranking years overall} \label{appx: wholerankings}
\end{textblock}

\begin{textblock}{0.89}[0,0](-0.27,0.01)
\begin{table*}[h]
\centering
\caption{Similarity between ranking years (O: Overlap; F: Spearmans correlation coefficient, M: M-measure).}
\label{table:Cross-similarity}
\begin{tabular*}{\textwidth}{l@{\extracolsep{\fill}}@{}cccccccccccccccccc}

\toprule
    
    Measure &
    \multicolumn{3}{c}{2012} &
    \multicolumn{3}{c}{2013} &
    \multicolumn{3}{c}{2014} &
    \multicolumn{3}{c}{2015} &
    \multicolumn{3}{c}{2016} &
    \multicolumn{3}{c}{2017} \\
    \cmidrule(lr){2-4}
    \cmidrule(lr){5-7}
    \cmidrule(lr){8-10}
    \cmidrule(lr){11-13}
    \cmidrule(lr){14-16}
    \cmidrule(lr){17-19}

    &
    O & F & M & O & F & M & O & F & M & O & F & M & O & F & M & O & F & M \\
    \midrule
    
    {\textbf{ARWU}} & & & & & & & & & \\
    2013 & 
489 & 0.99 & 0.97   \\
    
    2014 & 
467 & 0.95 & 0.96 &
473 & 0.96 & 0.95   \\
    
    2015 & 
468 & 0.94 & 0.96 &
472 & 0.95 & 0.95 &
485 & 0.99 & 0.98  \\
    
    2016 & 
440 & 0.87 & 0.9 &
446 & 0.88 & 0.92 &
458 & 0.94 & 0.93 &
459 & 0.95 & 0.93  \\
    
    2017 & 
432 & 0.87 & 0.89 &
438 & 0.88 & 0.89 &
448 & 0.94 & 0.92 &
449 & 0.94 & 0.92 &
467 & 0.97 & 0.94  \\
    
    2018 & 
432 & 0.86 & 0.88 &
434 & 0.87 & 0.88 &
443 & 0.93 & 0.91 &
444 & 0.94 & 0.91 &
459 & 0.96 & 0.93 &
471 & 0.98 & 0.97  \\ [1.5ex]
    
    {\textbf{THE}} & & & & & & & & & \\
    2013 & 
338 & 0.98 & 0.91   \\
    2014 & 
324 & 0.95 & 0.89 &
334 & 0.97 & 0.93   \\
    2015 & 
301 & 0.91 & 0.86 &
303 & 0.92 & 0.88 &
307 & 0.92 & 0.85   \\
    2016 & 
297 & 0.9 & 0.78 &
299 & 0.91 & 0.79 &
303 & 0.91 & 0.77 &
331 & 0.97 & 0.86   \\
    2017 & 
289 & 0.89 & 0.72 &
291 & 0.9 & 0.74 &
297 & 0.9 & 0.71 &
320 & 0.94 & 0.8 &
335 & 0.98 & 0.92  \\
    2018 & 
277 & 0.86 & 0.7 &
278 & 0.87 & 0.72 &
286 & 0.88 & 0.7 &
307 & 0.93 & 0.78 &
319 & 0.96 & 0.89 &
342 & 0.97 & 0.95 \\ [1.5ex]
     
    {\textbf{QS}} & & & & & & & & & \\
    2013 & 
376 & 0.99 & 0.92  \\
    2014 & 
370 & 0.97 & 0.89 &
384 & 0.99 & 0.91  \\
    2015 & 
368 & 0.95 & 0.83 &
373 & 0.96 & 0.88 &
371 & 0.96 & 0.85   \\
    2016 & 
359 & 0.94 & 0.82 &
365 & 0.95 & 0.84 &
364 & 0.96 & 0.84 &
381 & 0.99 & 0.94  \\
    2017 & 
357 & 0.93 & 0.81 &
361 & 0.94 & 0.83 &
361 & 0.95 & 0.82 &
375 & 0.98 & 0.91 &
384 & 0.98 & 0.96 \\
    2018 & 
354 & 0.91 & 0.8 &
356 & 0.92 & 0.8 &
357 & 0.93 & 0.8 &
367 & 0.96 & 0.88 &
374 & 0.97 & 0.93 &
383 & 0.99 & 0.95 \\
\bottomrule
\multicolumn{19}{l}{All Spearmans correlations (F) were significant: $p<.001$}\\
\multicolumn{19}{l}{For the ARWU the top 500 and for the THE and QS the top 400 universities are analysed}\\
\end{tabular*}
\end{table*}
When interpreting these results one has to take into account two considerations:
\begin{enumerate}
    \item Results for the ARWU and THE are largely based on re-calculated ranks. These ranks are not provided by the rankings
    \item For certain universities re-calculation because data was missing proved impossible. These were removed from the analysis.
\end{enumerate}
\end{textblock}
\clearpage

\begin{textblock}{0.89}[0,0](-0.27,-0.04)
\section{G. Similarity between different rankings overall} \label{appx: wholerankings}
\end{textblock}

\begin{textblock}{0.89}[0,0](-0.27,0.01)
\begin{table}[h]
\centering
\caption{Similarity between different rankings (O: Overlap; F: Spearman correlation coefficient; M: M-measure)}
\label{table:Within-similarity}
\begin{tabular}{lcccccc}

\toprule
    
    Measure &
    \multicolumn{6}{c}{Top 400} \\
    \cmidrule(lr){2-7}

    &
    \multicolumn{3}{c}{ARWU} &
    \multicolumn{3}{c}{THE} \\
    \cmidrule(lr){2-4}
    \cmidrule(lr){5-7}

    &
    O & F & M & O & F & M  \\
    \midrule
    
    {\textbf{2012}} \\
    THE & 
     270 & 0.74*** & 0.6
     & &  \\
    QS & 
301 & 0.67*** & 0.56 &
278 & 0.82*** & 0.57 \\ [1.5ex]
    
    {\textbf{2013}} \\
    THE & 
     273 & 0.72*** & 0.56
     & &  \\
    QS & 
309 & 0.68*** & 0.58 &
278 & 0.82*** & 0.57 \\ [1.5ex]
     
    {\textbf{2014}} \\
     THE & 
     275 & 0.73*** & 0.6
     & &  \\
    QS & 
302 & 0.67*** & 0.56 &
281 & 0.8*** & 0.56 \\ [1.5ex]
     
    {\textbf{2015}} \\
    THE & 
     276 & 0.72*** & 0.54
     & &  \\
    QS & 
299 & 0.63*** & 0.6 &
274 & 0.78*** & 0.59 \\ [1.5ex]
     
    {\textbf{2016}} \\
    THE & 
     272 & 0.75*** & 0.57
     & &  \\
    QS & 
291 & 0.66*** & 0.61 &
276 & 0.81*** & 0.6 \\ [1.5ex]
     
    {\textbf{2017}} \\
    THE & 
    267 & 0.74*** & 0.57
     & &  \\
    QS & 
288 & 0.67*** & 0.61 &
278 & 0.8*** & 0.6 \\ [1.5ex]
     
    {\textbf{2018}} \\
    THE & 
     270 & 0.74*** & 0.58
     & &  \\
    QS & 
290 & 0.67*** & 0.6 &
275 & 0.82*** & 0.61 \\
\bottomrule
\multicolumn{7}{l}{Note: * $p<.05$, ** $p<.01$, *** $p<.001$} \\
\end{tabular}
\end{table}
When interpreting these results one has to take into account two considerations:
\begin{enumerate}
    \item Results for the ARWU and THE are largely based on re-calculated ranks. These ranks are not provided by the rankings
    \item For certain universities re-calculation because data was missing proved impossible. These were removed from the analysis.
\end{enumerate}
\end{textblock}
